# Supplementary material for: Privacy-Preserving Ensemble Infused Enhanced Deep Neural Network Framework for Edge Cloud Convergence
Source: arXiv:2305.09224 source file (2023-05-16)
Supplement: Supplementary file 1 [file 06-appendix.tex]

\appendices

\section{}
Appendix one text goes here.

\section{}
Appendix two text goes here.
